# Supplementary material for: Challenges in determining whether ENSO is a damped or a self-sustained oscillation
Source: arXiv:2504.05513 source file (2026-12-03)
Supplement: Supplementary file 1 [file ENSODampedSelfSustained_SI_v1.pdf]

# Supporting Information for “Is ENSO a self-sustained or damped oscillation”

Elle Weeks<sup>1</sup>, Eli Tziperman<sup>1,2</sup>

<sup>1</sup>School of Engineering and Applied Sciences, Harvard University, Cambridge, Massachusetts

<sup>2</sup>Department of Earth and Planetary Sciences, Harvard University, Cambridge, Massachusetts

## Contents of this file

1. Figures S1 to S2

---

Corresponding author: E. M. Weeks, School of Engineering and Applied Sciences, Harvard University, Cambridge, MA, USA. (elleweeks@g.harvard.edu)

April 7, 2025, 1:33pm

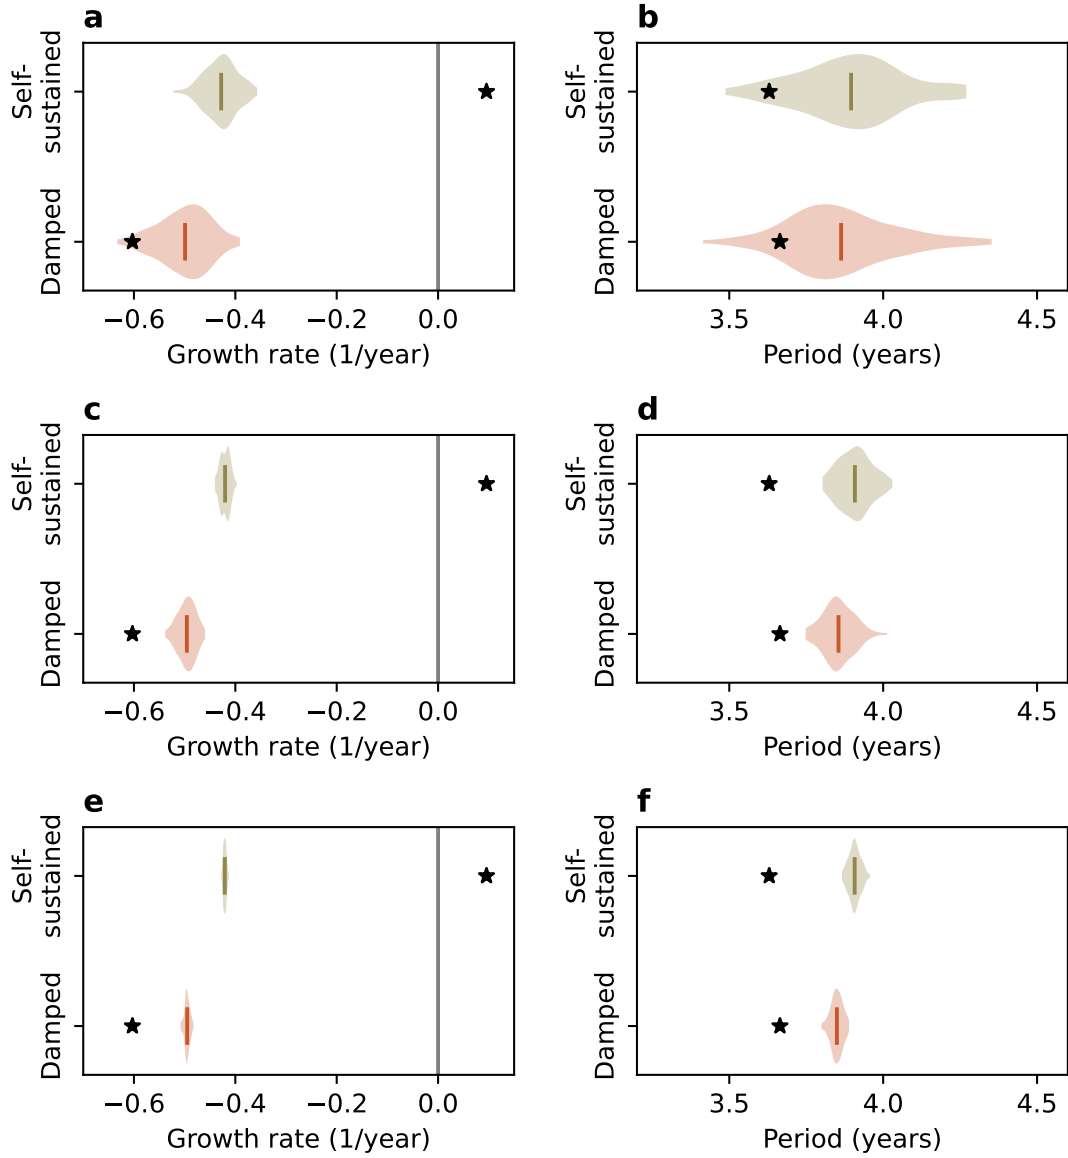

**Figure S1.** Estimates of the growth rate (left) and period (right) obtained by variations of fitting the RO equations to the simulated time series. Stars indicate the true parameter values. (a,b) Parameters estimated by fitting 100-year time series. (c,d) Parameters estimated by fitting 1,000-year time series. (e,f) Parameters estimated by fitting 10,000-year time series.

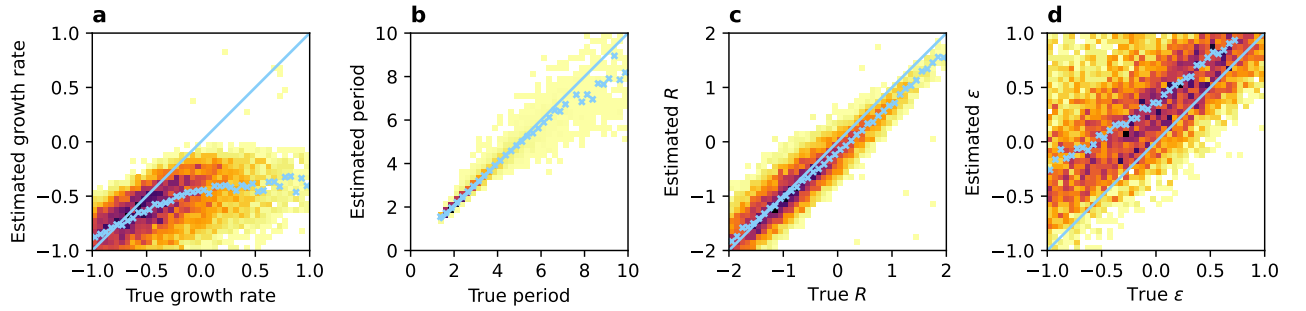

**Figure S2.** Comparison of estimates of the RO parameters—(a) growth rate, (b) period, (c)  $R$ , (d)  $\epsilon$ —obtained by fitting the NRO to the simulated time series with the true values. Time series were simulated according to the NRO with the cubic nonlinearity in the  $h$  equation instead of the  $T$  equation. Model parameters  $R$ ,  $\epsilon$ ,  $F_1$ , and  $F_2$  were varied across simulations. The one-to-one line is shown in blue.  $\times$ s indicate binned mean estimates.
